# Supplementary material for: PREEMPT: Proactive Robustness Evaluation under Editing for Media Protection Techniques
Source: arXiv:2610.24205 source file (2026-10-16)
Supplement: Supplementary file 2 [file 6_additional_analysis.tex]

\section{Additional Analysis}
\label{sec:additional_analysis}

To further validate the reasonableness of the proposed evaluation protocol, we conduct two additional analyses: (1) longer edit chains with depth $d=10$, and (2) mixed semantic edit chains.

\noindent\textbf{Sensitivity to Chain Length.} Our main experiments use edit chains with depth $d=4$, which provide a balance between evaluation cost and realistic editing scenarios. To address the concern that longer chains may exhibit substantially different behaviors, we further conduct an additional analysis with depth $d=10$. The longer heterogeneous chains consist of four semantic edits and six image-transformation-based edits. Note that this setting uses a different edit composition from the mixed chains in the main experiments and is not a direct extension of the $d=4$ setting.

As shown in Fig.~\ref{fig:curve_cx10_perturbation}, the degradation trends observed in the main experiments remain consistent under longer editing trajectories. Most perturbation-based methods continue to degrade gradually after the initial performance drop and reach the half-life threshold around depth 5--6. These results suggest that increasing the chain length mainly extends the degradation process rather than changing the overall conclusions. Therefore, the depth-4 setting used in the main experiments is sufficient to capture the primary robustness dynamics while keeping the evaluation cost manageable. Due to space limitations, the corresponding results for watermark-based methods are provided in the supplementary material.

\begin{figure}[htb]
    \centering
    \includegraphics[width=.95\linewidth]{fig/survival_curve_cx10_perturbation_ip2p.pdf}
    \caption{Protection survival curve of protection-based methods through 10-step heterogeneous edit chains.}
    \label{fig:curve_cx10_perturbation}
\end{figure}

\noindent\textbf{Mixed Semantic Chains.} 
To exclude the possibility that the observed degradation behavior is dominated by a particular semantic category, we further evaluate chains composed of mixed semantic edits. Specifically, each chain contains one edit from each semantic category following a fixed order: attribute, content, style, and spatial. The corresponding protection survival curves are shown in Fig.~\ref{fig:curve_c5}.

\begin{figure}[htb]
    \centering
    \includegraphics[width=0.9\linewidth]{fig/survival_c5_perturbation_ip2p.pdf}
    \caption{Protection survival curves under mixed semantic edit chains.}
    \label{fig:curve_c5}
\end{figure}

Similar trends to those observed in the homogeneous semantic chains are consistently reproduced. In particular, the largest performance drop still occurs after the first edit, while subsequent edits contribute comparatively smaller degradation. This result indicates that the rapid initial performance loss is a general characteristic of semantic editing rather than an artifact of any specific semantic category.
